# Supplementary material for: Detecting Conceptual Abstraction in LLMs
Source: arXiv:2404.15848 source file (2024-04-25)
Supplement: Supplementary file 1 [file appendix.tex]

\section{Dataset}\label{app:data}
We provide the datasets of test sentences along with the target and feature concepts as tsv files. There is one file for each of the three test sets ("positive.tsv", "negative.tsv", "sisters.tsv"). The files contain the following columns:
\begin{itemize}
    \item \textbf{id}: a running number unique over all example sentences
        \item \textbf{pattern}: the id of the pattern (cf. paper table)
        \item \textbf{text}: The example sentence
       \item \textbf{hyponym}: The string of the example sentence which refers to the hyponym in appropriately inflected form.
       \item \textbf{hypernym}	The word of the example sentence which refers to the hypernym, in inflected form. In the counterfactual settings, this is the matched term which has a type clash and is not actually a hypernym.
       \item \textbf{hyponym\_raw} The hyponym in base form.
       \item \textbf{hypernym\_raw}The hypernym in base form.
    
\end{itemize}

\section{Result visualisation}
\begin{figure*}[ht]
    \centering
    \begin{subfigure}{0.24\textwidth}
        \includegraphics[width=\linewidth]{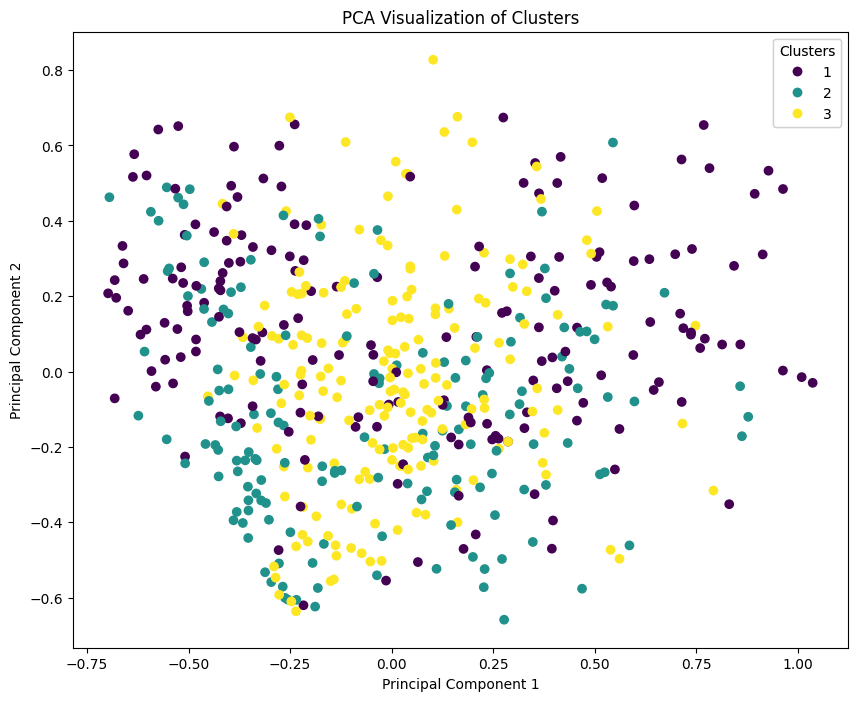}
        \caption{All datasets}
    \end{subfigure}
    \begin{subfigure}{0.24\textwidth}
        \includegraphics[width=\linewidth]{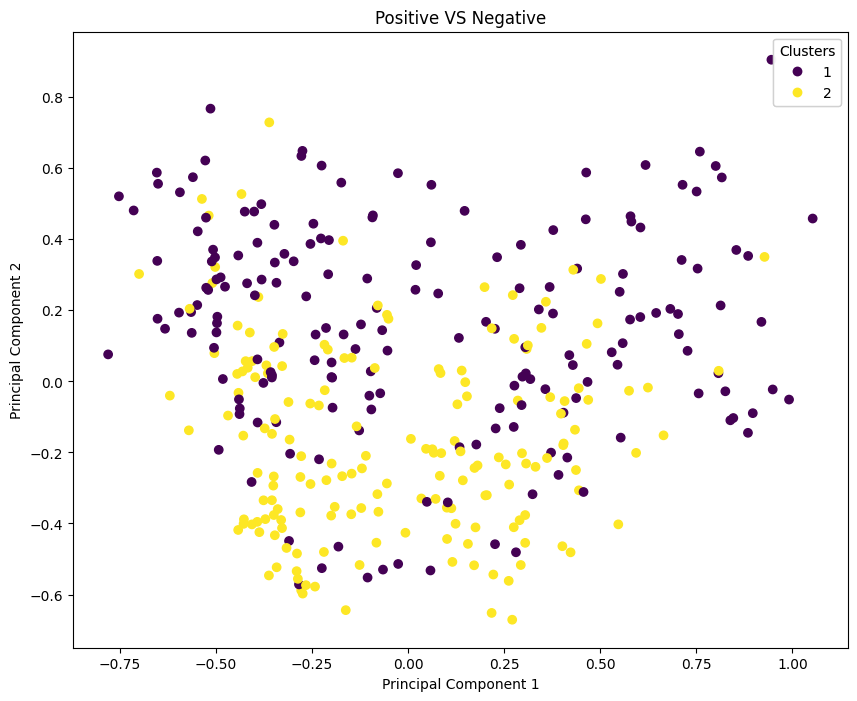}
        \caption{POS VS NEG}
    \end{subfigure}
    \vspace{0.5cm} % Add some vertical space between the rows of images
    \begin{subfigure}{0.24\textwidth}
        \includegraphics[width=\linewidth]{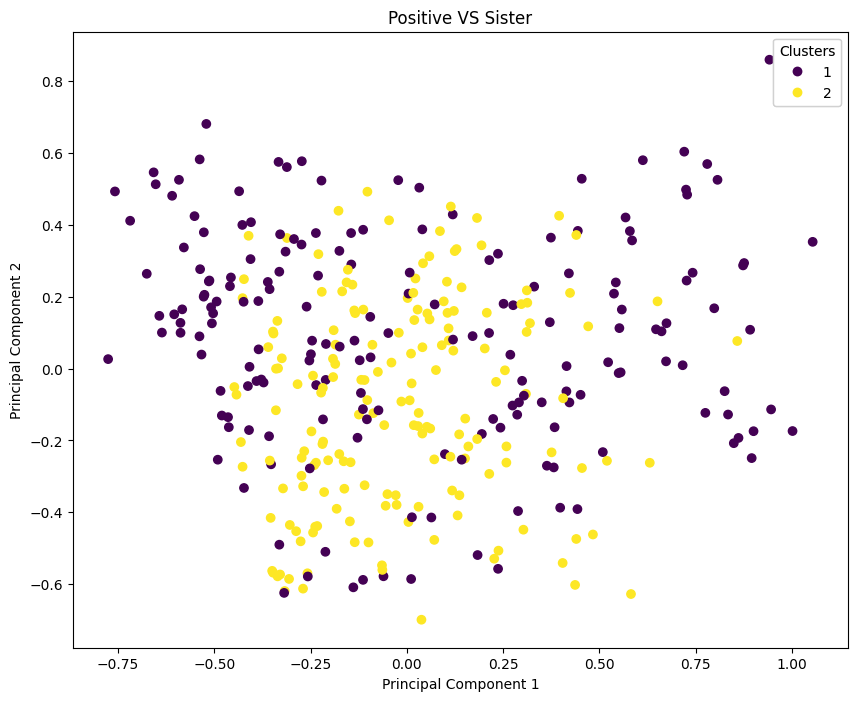}
        \caption{POS VS SIS}
    \end{subfigure}
    \begin{subfigure}{0.24\textwidth}
        \includegraphics[width=\linewidth]{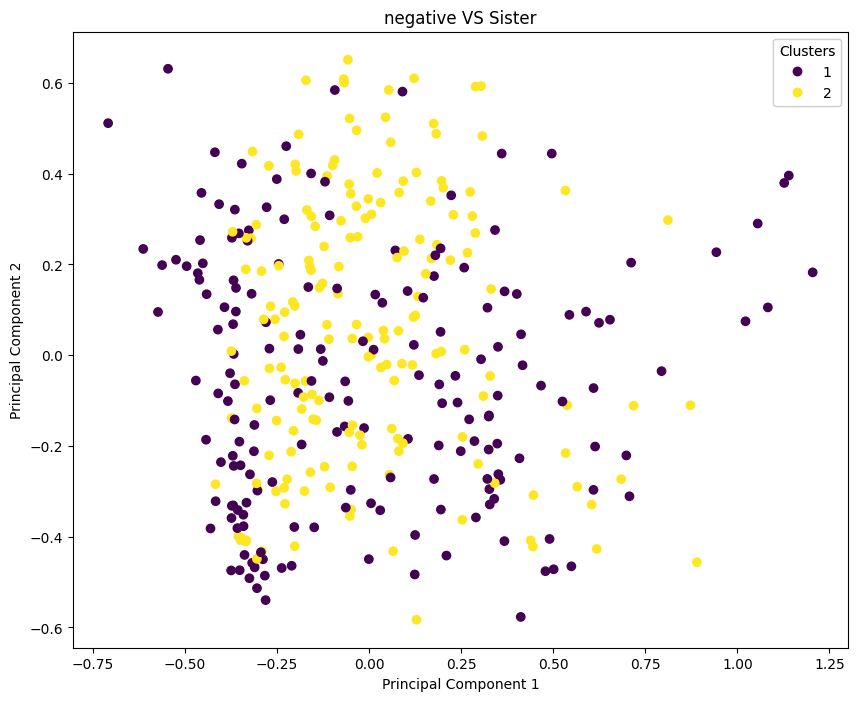}
        \caption{NEG VS SIS}
    \end{subfigure}
    \caption{Four images in a two-column document.}
\end{figure*}
\section{Example Appendix}
\label{sec:appendix}

This is an appendix.

 \textcolor{red}{Throwing everything here}

\section{Tokenization of Example sentences}\label{att:tokenization}
We use the attention from our target tokens to our feature tokens, and vice versa. In our patterns, those tokens have different sequential positions. In order not to hardcode every sentence, all sentences in each pattern must follow a structure where the hyponym and hypernym must exist in the token position given in Table \ref{tab:tokenRules}. 
The reason we retrieve negative tokens for hypernyms is that we can retreive the correct hypernym (backwards) and also retrieve the correct hyponym (without s). So we can leverage as much data as we can from the dataset.
\begin{table}[httb]
    \centering
    \begin{tabular}{lcccc}
    \toprule
         Patterns & Positive & Negative & Sister\\
         \midrule
        Pattern 1&129 & 129 & 129  \\
        Pattern 2& 236 & 236 & 236 \\
        Pattern 3& 158 & 158 & 158 \\
        Pattern 4& 236 & 236 & 236 \\
        Pattern 5& 128 & 128 & 128 \\
         \bottomrule
    \end{tabular}
    \captionsetup{width=0.9\textwidth} % adjust the width as needed
    \caption{Number of sentences for each dataset per pattern.}
    \label{tab:numberOfSentences}
\end{table}

\begin{table*}[httb]
    \centering
    \begin{tabular}{lcccc}
    \toprule
         Patterns & Positive example & Source Token & Target token\\
         \midrule
        Pattern 1&alligators are reptiles.& Token [1] & Token [-3]  \\
        Pattern 2& That hammer is a tool. & Token [2] & Token [-3] \\
        Pattern 3& I like hawks and other predators.& Token [3] & Token [-3] \\
        Pattern 4& The pear, which was the largest fruit among them, stood out.& Token [2] & Token [-8] \\
        Pattern 5& I like cherrys, particularly because they are fruit. & Token [3] & Token [-3] \\
         \bottomrule
    \end{tabular}
    
    \captionsetup{width=0.9\textwidth} % adjust the width as needed
    \caption{Which tokens are attended per pattern.}
    \label{tab:tokenRules}
\end{table*}

\begin{table}[httb]
    \centering
    \begin{tabular}{lcccc}
    \toprule
         Sentence &Tokenization\\
         \midrule
        clocks are watches.& 'clocks', 'are', 'watches', '.' \\
        harmonicas are musical instruments.&'harmonica', '\#\#s', 'are', 'musical', 'instruments', '.' \\
        grasshoppers are insects.& 'grass', '\#\#hopper', '\#\#s', 'are', 'insects', '.' \\
        harpoons are weapons.& 'harp', '\#\#oons', 'are', 'weapons', '.'\\
        gophers are animals.&'go', '\#\#pher', '\#\#s', 'are', 'animals', '.'\\
         \bottomrule
    \end{tabular}
    \captionsetup{width=0.9\textwidth} % adjust the width as needed
    \caption{Examples of different BERT tokenizations.}
    \label{tab:numberOfSentences}
\end{table}

\begin{figure*}
    \centering
    \begin{subfigure}{0.32\textwidth}
        \includegraphics[width=\linewidth]{LRECCOLING2024/Figures/Pattern1/P1_FP.png}
        \caption{Forward positive}
    \end{subfigure}
    \begin{subfigure}{0.32\textwidth}
        \includegraphics[width=\linewidth]{LRECCOLING2024/Figures/Pattern1/P1_BP.png}
        \caption{backward positive}
    \end{subfigure}
    \vspace{0.5cm} % Add some vertical space between the rows of images
    \begin{subfigure}{0.32\textwidth}
        \includegraphics[width=\linewidth]{LRECCOLING2024/Figures/Pattern1/P1_AP.png}
        \caption{Average positive}
    \end{subfigure}
    \begin{subfigure}{0.32\textwidth}
        \includegraphics[width=\linewidth]{LRECCOLING2024/Figures/Pattern1/P1_FN.png}
        \caption{Forward negative}
    \end{subfigure}
    \begin{subfigure}{0.32\textwidth}
        \includegraphics[width=\linewidth]{LRECCOLING2024/Figures/Pattern1/P1_BN.png}
        \caption{Backward negative}
    \end{subfigure}
    \begin{subfigure}{0.32\textwidth}
        \includegraphics[width=\linewidth]{LRECCOLING2024/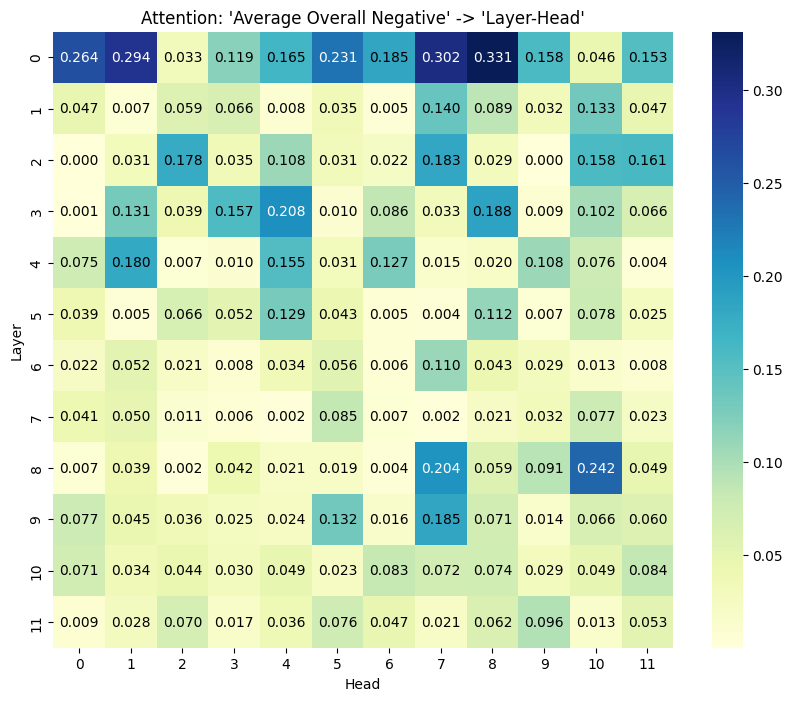}
        \caption{Average negative}
    \end{subfigure}
    \begin{subfigure}{0.32\textwidth}
        \includegraphics[width=\linewidth]{LRECCOLING2024/Figures/Pattern1/P1_FS.png}
        \caption{Forward sister}
    \end{subfigure}
\begin{subfigure}{0.32\textwidth}
        \includegraphics[width=\linewidth]{LRECCOLING2024/Figures/Pattern1/P1_BS.png}
        \caption{Backward sister}
    \end{subfigure}
\begin{subfigure}{0.32\textwidth}
        \includegraphics[width=\linewidth]{LRECCOLING2024/Figures/Pattern1/P1_AS.png}
        \caption{Average sister}
    \end{subfigure}
    \caption{Attention maps for hyponyms and hypernyms across all heads for Pattern 1.}
\end{figure*}

\begin{figure*}
    \centering
    \begin{subfigure}{0.32\textwidth}
        \includegraphics[width=\linewidth]{LRECCOLING2024/Figures/Pattern1/P1_first_skew.png}
        \caption{Skewness of first layer}
    \end{subfigure}
    \begin{subfigure}{0.32\textwidth}
        \includegraphics[width=\linewidth]{LRECCOLING2024/Figures/Pattern1/P1_last_skew.png}
        \caption{Skewness of last layer}
    \end{subfigure}
    \vspace{0.5cm} % Add some vertical space between the rows of images

    \caption{Skewness for first and last layer in pattern1.}
\end{figure*}

\begin{figure*}[ht]
    \centering
    \begin{subfigure}{0.32\textwidth}
        \includegraphics[width=\linewidth]{LRECCOLING2024/Figures/Pattern2/P2_FP.png}
        \caption{Forward positive}
    \end{subfigure}
    \begin{subfigure}{0.32\textwidth}
        \includegraphics[width=\linewidth]{LRECCOLING2024/Figures/Pattern2/P2_BP.png}
        \caption{backward positive}
    \end{subfigure}
    \vspace{0.5cm} % Add some vertical space between the rows of images
    \begin{subfigure}{0.32\textwidth}
        \includegraphics[width=\linewidth]{LRECCOLING2024/Figures/Pattern2/P2_AP.png}
        \caption{Average positive}
    \end{subfigure}
    \begin{subfigure}{0.32\textwidth}
        \includegraphics[width=\linewidth]{LRECCOLING2024/Figures/Pattern2/P2_FN.png}
        \caption{Forward negative}
    \end{subfigure}
    \begin{subfigure}{0.32\textwidth}
        \includegraphics[width=\linewidth]{LRECCOLING2024/Figures/Pattern2/P2_BN.png}
        \caption{Backward negative}
    \end{subfigure}
    \begin{subfigure}{0.32\textwidth}
        \includegraphics[width=\linewidth]{LRECCOLING2024/Figures/Pattern2/P2_AN.png}
        \caption{Average negative}
    \end{subfigure}
    \begin{subfigure}{0.32\textwidth}
        \includegraphics[width=\linewidth]{LRECCOLING2024/Figures/Pattern2/P2_FS.png}
        \caption{Forward sister}
    \end{subfigure}
\begin{subfigure}{0.32\textwidth}
        \includegraphics[width=\linewidth]{LRECCOLING2024/Figures/Pattern2/P2_BS.png}
        \caption{Backward sister}
    \end{subfigure}
\begin{subfigure}{0.32\textwidth}
        \includegraphics[width=\linewidth]{LRECCOLING2024/Figures/Pattern2/P2_AS.png}
        \caption{Average sister}
    \end{subfigure}
    \caption{Attention maps for hyponyms and hypernyms across all heads for Pattern 2.}
\end{figure*}

\begin{figure*}
    \centering
    \begin{subfigure}{0.32\textwidth}
        \includegraphics[width=\linewidth]{LRECCOLING2024/Figures/Pattern2/P2_first_skew.png}
        \caption{Skewness of first layer}
    \end{subfigure}
    \begin{subfigure}{0.32\textwidth}
        \includegraphics[width=\linewidth]{LRECCOLING2024/Figures/Pattern2/P2_last_skew.png}
        \caption{Skewness of last layer}
    \end{subfigure}
    \vspace{0.5cm} % Add some vertical space between the rows of images

    \caption{Skewness for first and last layer in pattern1.}
\end{figure*}

\begin{figure*}[ht]
    \centering
    \begin{subfigure}{0.32\textwidth}
        \includegraphics[width=\linewidth]{LRECCOLING2024/Figures/Pattern3/P3_FP.png}
        \caption{Forward positive}
    \end{subfigure}
    \begin{subfigure}{0.32\textwidth}
        \includegraphics[width=\linewidth]{LRECCOLING2024/Figures/Pattern3/P3_BP.png}
        \caption{backward positive}
    \end{subfigure}
    \vspace{0.5cm} % Add some vertical space between the rows of images
    \begin{subfigure}{0.32\textwidth}
        \includegraphics[width=\linewidth]{LRECCOLING2024/Figures/Pattern3/P3_AP.png}
        \caption{Average positive}
    \end{subfigure}
    \begin{subfigure}{0.32\textwidth}
        \includegraphics[width=\linewidth]{LRECCOLING2024/Figures/Pattern3/P3_FN.png}
        \caption{Forward negative}
    \end{subfigure}
    \begin{subfigure}{0.32\textwidth}
        \includegraphics[width=\linewidth]{LRECCOLING2024/Figures/Pattern3/P3_BN.png}
        \caption{Backward negative}
    \end{subfigure}
    \begin{subfigure}{0.32\textwidth}
        \includegraphics[width=\linewidth]{LRECCOLING2024/Figures/Pattern3/P3_AN.png}
        \caption{Average negative}
    \end{subfigure}
    \begin{subfigure}{0.32\textwidth}
        \includegraphics[width=\linewidth]{LRECCOLING2024/Figures/Pattern3/P3_FS.png}
        \caption{Forward sister}
    \end{subfigure}
\begin{subfigure}{0.32\textwidth}
        \includegraphics[width=\linewidth]{LRECCOLING2024/Figures/Pattern3/P3_BS.png}
        \caption{Backward sister}
    \end{subfigure}
\begin{subfigure}{0.32\textwidth}
        \includegraphics[width=\linewidth]{LRECCOLING2024/Figures/Pattern3/P3_AS.png}
        \caption{Average sister}
    \end{subfigure}
    \caption{Attention maps for hyponyms and hypernyms across all heads for Pattern 3.}
\end{figure*}

\begin{figure*}
    \centering
    \begin{subfigure}{0.32\textwidth}
        \includegraphics[width=\linewidth]{LRECCOLING2024/Figures/Pattern3/P3_first_skew.png}
        \caption{Skewness of first layer}
    \end{subfigure}
    \begin{subfigure}{0.32\textwidth}
        \includegraphics[width=\linewidth]{LRECCOLING2024/Figures/Pattern3/P3_last_skew.png}
        \caption{Skewness of last layer}
    \end{subfigure}
    \vspace{0.5cm} % Add some vertical space between the rows of images

    \caption{Skewness for first and last layer in pattern3}
\end{figure*}

\begin{figure*}[ht]
    \centering
    \begin{subfigure}{0.32\textwidth}
        \includegraphics[width=\linewidth]{LRECCOLING2024/Figures/Pattern4/P4_FP.png}
        \caption{Forward positive}
    \end{subfigure}
    \begin{subfigure}{0.32\textwidth}
        \includegraphics[width=\linewidth]{LRECCOLING2024/Figures/Pattern4/P4_BP.png}
        \caption{backward positive}
    \end{subfigure}
    \vspace{0.5cm} % Add some vertical space between the rows of images
    \begin{subfigure}{0.32\textwidth}
        \includegraphics[width=\linewidth]{LRECCOLING2024/Figures/Pattern4/P4_AP.png}
        \caption{Average positive}
    \end{subfigure}
    \begin{subfigure}{0.32\textwidth}
        \includegraphics[width=\linewidth]{LRECCOLING2024/Figures/Pattern4/P4_FN.png}
        \caption{Forward negative}
    \end{subfigure}
    \begin{subfigure}{0.32\textwidth}
        \includegraphics[width=\linewidth]{LRECCOLING2024/Figures/Pattern4/P4_BN.png}
        \caption{Backward negative}
    \end{subfigure}
    \begin{subfigure}{0.32\textwidth}
        \includegraphics[width=\linewidth]{LRECCOLING2024/Figures/Pattern4/P4_AN.png}
        \caption{Average negative}
    \end{subfigure}
    \begin{subfigure}{0.32\textwidth}
        \includegraphics[width=\linewidth]{LRECCOLING2024/Figures/Pattern4/P4_FS.png}
        \caption{Forward sister}
    \end{subfigure}
\begin{subfigure}{0.32\textwidth}
        \includegraphics[width=\linewidth]{LRECCOLING2024/Figures/Pattern4/P4_BS.png}
        \caption{Backward sister}
    \end{subfigure}
\begin{subfigure}{0.32\textwidth}
        \includegraphics[width=\linewidth]{LRECCOLING2024/Figures/Pattern4/P4_AS.png}
        \caption{Average sister}
    \end{subfigure}
    \caption{Attention maps for hyponyms and hypernyms across all heads for Pattern 4.}
\end{figure*}

\begin{figure*}
    \centering
    \begin{subfigure}{0.32\textwidth}
        \includegraphics[width=\linewidth]{LRECCOLING2024/Figures/Pattern4/P4_first_skew.png}
        \caption{Skewness of first layer}
    \end{subfigure}
    \begin{subfigure}{0.32\textwidth}
        \includegraphics[width=\linewidth]{LRECCOLING2024/Figures/Pattern4/P4_last_skew.png}
        \caption{Skewness of last layer}
    \end{subfigure}
    \vspace{0.5cm} % Add some vertical space between the rows of images

    \caption{Skewness for first and last layer in pattern4}
\end{figure*}

\begin{figure*}[ht]
    \centering
    \begin{subfigure}{0.32\textwidth}
        \includegraphics[width=\linewidth]{LRECCOLING2024/Figures/Pattern5/P5_FP.png}
        \caption{Forward positive}
    \end{subfigure}
    \begin{subfigure}{0.32\textwidth}
        \includegraphics[width=\linewidth]{LRECCOLING2024/Figures/Pattern5/P5_BP.png}
        \caption{backward positive}
    \end{subfigure}
    \vspace{0.5cm} % Add some vertical space between the rows of images
    \begin{subfigure}{0.32\textwidth}
        \includegraphics[width=\linewidth]{LRECCOLING2024/Figures/Pattern5/P5_AP.png}
        \caption{Average positive}
    \end{subfigure}
    \begin{subfigure}{0.32\textwidth}
        \includegraphics[width=\linewidth]{LRECCOLING2024/Figures/Pattern5/P5_FN.png}
        \caption{Forward negative}
    \end{subfigure}
    \begin{subfigure}{0.32\textwidth}
        \includegraphics[width=\linewidth]{LRECCOLING2024/Figures/Pattern5/P5_BN.png}
        \caption{Backward negative}
    \end{subfigure}
    \begin{subfigure}{0.32\textwidth}
        \includegraphics[width=\linewidth]{LRECCOLING2024/Figures/Pattern5/P5_AN.png}
        \caption{Average negative}
    \end{subfigure}
    \begin{subfigure}{0.32\textwidth}
        \includegraphics[width=\linewidth]{LRECCOLING2024/Figures/Pattern5/P5_FS.png}
        \caption{Forward sister}
    \end{subfigure}
\begin{subfigure}{0.32\textwidth}
        \includegraphics[width=\linewidth]{LRECCOLING2024/Figures/Pattern5/P5_BS.png}
        \caption{Backward sister}
    \end{subfigure}
\begin{subfigure}{0.32\textwidth}
        \includegraphics[width=\linewidth]{LRECCOLING2024/Figures/Pattern5/P5_AS.png}
        \caption{Average sister}
    \end{subfigure}
    \caption{Attention maps for hyponyms and hypernyms across all heads for Pattern 5.}
\end{figure*}

\begin{figure*}
    \centering
    \begin{subfigure}{0.32\textwidth}
        \includegraphics[width=\linewidth]{LRECCOLING2024/Figures/Pattern5/P5_first_skew.png}
        \caption{Skewness of first layer}
    \end{subfigure}
    \begin{subfigure}{0.32\textwidth}
        \includegraphics[width=\linewidth]{LRECCOLING2024/Figures/Pattern5/P5_last_skew.png}
        \caption{Skewness of last layer}
    \end{subfigure}
    \vspace{0.5cm} % Add some vertical space between the rows of images

    \caption{Skewness for first and last layer in pattern5}
\end{figure*}

\begin{figure*}[ht]
    \centering
    \begin{subfigure}{0.32\textwidth}
        \includegraphics[width=\linewidth]{LRECCOLING2024/Figures/All Patterns/ALL_FP.png}
        \caption{Forward positive}
    \end{subfigure}
    \begin{subfigure}{0.32\textwidth}
        \includegraphics[width=\linewidth]{LRECCOLING2024/Figures/All Patterns/ALL_BP.png}
        \caption{backward positive}
    \end{subfigure}
    \vspace{0.5cm} % Add some vertical space between the rows of images
    \begin{subfigure}{0.32\textwidth}
        \includegraphics[width=\linewidth]{LRECCOLING2024/Figures/All Patterns/ALL_AP.png}
        \caption{Average positive}
    \end{subfigure}
    \begin{subfigure}{0.32\textwidth}
        \includegraphics[width=\linewidth]{LRECCOLING2024/Figures/All Patterns/ALL_FN.png}
        \caption{Forward negative}
    \end{subfigure}
    \begin{subfigure}{0.32\textwidth}
        \includegraphics[width=\linewidth]{LRECCOLING2024/Figures/All Patterns/ALL_BN.png}
        \caption{Backward negative}
    \end{subfigure}
    \begin{subfigure}{0.32\textwidth}
        \includegraphics[width=\linewidth]{LRECCOLING2024/Figures/All Patterns/ALL_AN.png}
        \caption{Average negative}
    \end{subfigure}
    \begin{subfigure}{0.32\textwidth}
        \includegraphics[width=\linewidth]{LRECCOLING2024/Figures/All Patterns/ALL_FS.png}
        \caption{Forward sister}
    \end{subfigure}
\begin{subfigure}{0.32\textwidth}
        \includegraphics[width=\linewidth]{LRECCOLING2024/Figures/All Patterns/ALL_BS.png}
        \caption{Backward sister}
    \end{subfigure}
\begin{subfigure}{0.32\textwidth}
        \includegraphics[width=\linewidth]{LRECCOLING2024/Figures/All Patterns/ALL_AS.png}
        \caption{Average sister}
    \end{subfigure}
    \caption{Attention maps for hyponyms and hypernyms averaged across all patterns.}
\end{figure*}

\begin{figure*}
	 \centerline{\includegraphics[width=0.65\textwidth]{LRECCOLING2024/Figures/All Patterns/Average skewness across all patterns.png}}
	 {\caption{Average Skewness across all patterns}}
\end{figure*}
